# Supplementary material for: Dynamical Phonons Following Electron Relaxation Stages in Photo-excited Graphene
Source: arXiv:2309.09076 ancillary file (2023-09-16)
Supplement: Supplementary file 1 [file Supplemental_Material__NEQ_gr___Nano_Lett_-1.pdf]

# Supporting information for:

# Dynamical Phonons Following Electron Relaxation Stages in Photo-excited Graphene

Nina Girotto and Dino Novko*

*Centre for Advanced Laser Techniques, Institute of Physics, 10000 Zagreb, Croatia*

E-mail: dino.novko@gmail.com

## S1 Computational details

In this work, we explicitly focus on the non-equilibrium carrier distribution scattering on phonons and analyze how the different stages of transient distribution affect the EPC properties deriving from the phonon self-energy [S1]

$$\pi_{\nu}^{c}(\mathbf{q},\omega) = \sum_{\mathbf{k}nm} \left|g_{\nu}^{nm,c}(\mathbf{k},\mathbf{q})\right|^{2} \frac{f_{n\mathbf{k}}^{c} - f_{m\mathbf{k+q}}^{c}}{\varepsilon_{n\mathbf{k}}^{c} - \varepsilon_{m\mathbf{k+q}}^{c} + \omega + i\eta}. \tag{S1}$$

Here $g_{\nu}^{nm,c}(\mathbf{k},\mathbf{q})$ denotes the EPC matrix elements, $\varepsilon_{n\mathbf{k}}^{c}$ are the Kohn-Sham energies, and $f_{n\mathbf{k}}^{c}$ are the electron occupation functions. $n$ and $m$ are the electron band indices, $\nu$ is the phonon index, while $\mathbf{k}$ and $\mathbf{q}$ are electron and phonon wavevectors. The superscript "$c$" denotes the quantities which are modified in cDFPT. We model the out-of-equilibrium electron distribution [see Fig. 1(b-c) of the main text] as an equilibrium Fermi-Dirac distribution with the addition and subtraction of Gaussian packets. Imposing an arbitrary (e.g., nonequilibrium) distribution $n(\varepsilon)$ of Dirac fermions, was already done for several 2D materials in order to investigate the linear response under non-Fermi-Dirac

conditions [S2,S3]. The general expression for the photo-excited distribution in our model is

$$n(\varepsilon) = f(\varepsilon)|_{E_F}^{T} - \delta_1 e^{\frac{(\frac{\varepsilon_1-\varepsilon_2}{2}-\varepsilon_1+\varepsilon)^2}{\alpha(\varepsilon_1-\varepsilon_2)}} + \delta_2 e^{\frac{(\frac{\varepsilon_3-\varepsilon_4}{2}-\varepsilon_3+\varepsilon)^2}{\alpha(\varepsilon_3-\varepsilon_4)}} \tag{S2}$$

where all the energies are measured with respect to the Fermi energy $E_F$ in dimensionless units (divided by the electronic temperature or the smearing value). $f(\varepsilon)|_{E_F}^{T}$ denotes the equilibrium Fermi-Dirac distribution at temperature $T$, i.e., $f(\varepsilon)|_{E_F}^{T} = \left(1 + e^{\frac{\varepsilon - E_F}{k_B T}}\right)^{-1}$, with $k_B$ being the Boltzmann factor. The addition (subtraction) of the Gaussian term represents the development of the carrier (hole) population in the conduction (valence) band. Energies $\varepsilon_x$ are marked in Fig. 1(b), and since the laser pulse has a vanishing momentum, we set $-\varepsilon_1 = \varepsilon_4$ and $-\varepsilon_2 = \varepsilon_3$. Factor $\alpha$ is present to ensure that the added (subtracted) population is confined in the desired energy interval. Factors $\delta_{1,2}$ are chosen so that the two claims hold true: (i) distribution $n(\varepsilon)$ never exceeds 1, or reduces below 0, and (ii) the total number of photo-holes and photo-electrons is preserved. The case of photo-inversion [Fig. 1(c)] is the limiting case of Eq. (S2), where $\varepsilon_2 = \varepsilon_3 = 0$.

We calculate the equilibrium number of carriers $N_e$, characterized by the Fermi-Dirac distribution using the density of states $N(\varepsilon)$ like

$$N_e = \int_{\varepsilon_D}^{\infty} d\varepsilon N(\varepsilon) f(\varepsilon)|_{E_F}^{T_e}.$$

Then, we modify the Fermi- Dirac distribution to a photo-excited distribution $n(\varepsilon)$ and vary it in order to conserve the number of carriers. In other words, the condition

$$N_e = \int_{\varepsilon_D}^{\infty} d\varepsilon N(\varepsilon) n(\varepsilon)$$

needs to be satisfied. Note that as the free parameters we consider either $\varepsilon_1$ and $\varepsilon_2$ or their equivalent above the Dirac point ($\varepsilon_{3,4}$), but not both. The carrier number conservation is finally ensured with the factors $\delta_{1,2}$ from the expression (S2). In the case of a hot electron distribution, the same logic applies. The number of photo-excited carriers becomes the number of carriers above the Dirac point

described by a hot Fermi-Dirac distribution with a corresponding electron temperature. For our set of parameters, the electronic temperature for which the number of carriers remains consistent is 2200 K. In the case of a photo-excited and photo-inverted calculation we manually change the Fermi-Dirac distribution in the self-consistent DFT calculation. The modified distribution then enters the DFPT calculation. In DFPT, the change of the self-consistent potential due to the ionic displacements $\Delta V_{SCF}$ needs to be calculated like

$$\Delta V_{SCF} = \Delta V_{ion}(\mathbf{r}) + e^2 \int \frac{\Delta n(\mathbf{r})}{|\mathbf{r} - \mathbf{r}'|} d\mathbf{r}' + \frac{dV_{xc}[n]}{dn}|_{n=n_0(\mathbf{r})} \Delta n(\mathbf{r}). \tag{S3}$$

It is determined as a sum of three terms; the change of the ionic potential, the Hartree screening contribution and exchange contribution. $\Delta V_{SCF}$ contains electron density response $\Delta n(\mathbf{r})$ to the ionic displacement, which can be obtained as

$$\Delta n(\mathbf{r}) = \sum_{n,m} \frac{f(\varepsilon_n)|_{E_F}^{T_e} - f(\varepsilon_m)|_{E_F}^{T_e}}{\varepsilon_n - \varepsilon_m} \psi_n^*(\mathbf{r}) \psi_m(\mathbf{r}) \langle \psi_m | \Delta V_{SCF} | \psi_n \rangle \tag{S4}$$

where the Kohn-Sham states are denoted by $\psi(\mathbf{r})$. In order to avoid the summation over the unoccupied states, in DFPT the equations being solved are[S4]:

$$(H_{SCF} + Q - \varepsilon_n) |\Delta\psi_n\rangle = -(f(\varepsilon_n)|_{E_F}^{T_e} - P_n) \Delta V_{SCF} |\psi_n\rangle \tag{S5}$$

where

$$Q = \sum_m \alpha_m |\psi_m\rangle \langle\psi_m|$$

,

$$P_n = \sum_m \beta_{n,m} |\psi_m\rangle \langle\psi_m|$$

$$\Delta\psi_n = \sum_m \frac{f(\varepsilon_n)|_{E_F}^{T_e} - f(\varepsilon_m)|_{E_F}^{T_e}}{\varepsilon_n - \varepsilon_m} f(\varepsilon_n)|_{\varepsilon_m}^{T_e} \psi_m(\mathbf{r}) \langle \psi_m | \Delta V_{SCF} | \psi_n \rangle$$

and

$$\beta_{n,m} = f(\varepsilon_n)|_{E_F}^{T_e} f(\varepsilon_m)|_{\varepsilon_n}^{T_e} + f(\varepsilon_m)|_{E_F}^{T_e} f(\varepsilon_n)|_{\varepsilon_m}^{T_e} + \alpha_m \frac{f(\varepsilon_n)|_{E_F}^{T_e} - f(\varepsilon_m)|_{E_F}^{T_e}}{\varepsilon_n - \varepsilon_m} f(\varepsilon_n)|_{\varepsilon_m}^{T_e}.$$

The parameters $\alpha_m$ are present in order to avoid zero eigenvalues of the matrix on the left-hand side of the equation $(H_{SCF} + Q - \varepsilon_n)$. Note that in DFT, the Fermi- Dirac distribution can be exchanged by any suitable equivalent available in the code. Since in our approach the Fermi-Dirac distribution is exchanged by an excited distribution $n(\varepsilon)$ from Eq. (S2), the expression for $\beta_{n,m}$ is changed accordingly, introducing the photo-excited (or photo-inverted) distribution of electrons in the phonon calculation. Spectral function is calculated by using the following expression [S1]

$$B^c_\nu(\mathbf{q},\omega) = -\frac{1}{\pi}\mathrm{Im}\left\{\frac{2\omega^c_{\mathbf{q}\nu}}{\omega^2 - (\omega^c_{\mathbf{q}\nu})^2 - 2\omega^c_{\mathbf{q}\nu}[\pi^c_\nu(\mathbf{q},\omega) - \pi^c_\nu(\mathbf{q})]}\right\}. \tag{S6}$$

We subtract the adiabatic phonon self-energy on a coarse mesh, used in the PHonon [S4,S5] calculation. The nonadiabatic frequencies can be obtained as $\Omega^2_{\mathbf{q}\nu} = \omega^2_{\mathbf{q}\nu} + 2\omega_{\mathbf{q}\nu}\mathrm{Re}\,\pi_\nu(\mathbf{q},\Omega_{\mathbf{q}\nu})$ and the corresponding linewidths as $\gamma_{\mathbf{q}\nu} = -\mathrm{Im}\,\pi_\nu(\mathbf{q},\Omega_{\mathbf{q}\nu})$.

In order to analyze different contributions to the phonon renormalization we simplify the adiabatic phonon self-energy as calculated in cDFPT as [S6,S7]

$$\pi^c_\nu(\mathbf{q}) = \sum_{\mathbf{k}nm}\left|g^{nm,c}_\nu(\mathbf{k},\mathbf{q})\right|^2\frac{f^c_{n\mathbf{k}} - f^c_{m\mathbf{k}+\mathbf{q}}}{\varepsilon^c_{n\mathbf{k}} - \varepsilon^c_{m\mathbf{k}+\mathbf{q}}} \approx |g^c_\nu(\mathbf{q})|^2\sum_{\mathbf{k}nm}\frac{f^c_{n\mathbf{k}} - f^c_{m\mathbf{k}+\mathbf{q}}}{\varepsilon^c_{n\mathbf{k}} - \varepsilon^c_{m\mathbf{k}+\mathbf{q}}} = |g^c_\nu(\mathbf{q})|^2\chi^c_0(\mathbf{q}), \tag{S7}$$

where we averaged out the electronic degrees of freedom deriving from the EPC matrix elements, leading to $|g^{nm,c}_\nu(\mathbf{k},\mathbf{q})| \rightarrow |g^c_\nu(\mathbf{q})|$. With this we can disentangle the purely phase space contributions coming from $\chi^0(\mathbf{q})$ and the electron-phonon contributions coming from the effective coupling $|g^c_\nu(\mathbf{q})|^2$.

For the density functional theory (DFT) calculations, we use QUANTUM ESPRESSO[S5] and for EPC we use the EPW code[S8]. We use the norm-conserving scalar pseudopotential from the PSEUDODOJO table[S9] with an energy cutoff of 100 Ry. The relaxed lattice constant is 2.449 Å and the periodic graphene planes are separated by 12 Å. We use Fermi-Dirac smearing with $T = 800$ K. When modifying the electron distribution, we do not relax the structure, since we assume that the structure relaxation timescale is larger than the timescales we are interested in this work. In order to capture all the relevant transitions, we densely sampled the Brillouin zone with a uniform coarse

$60 \times 60 \times 1$ k-mesh. The phonon calculation [S4] is done on a uniform coarse $12 \times 12 \times 1$ q-mesh. For the EPC calculation, the starting point is the Wannierization. We use maximally localized Wannier functions[S10], with five initial projections corresponding to one $sp^2$ orbital and two $p_z$ orbitals on C atom sites. The resulting Wannier functions lie on top of the two C atoms from the unit cell and on the bond centers. Smearing in the EPW calculation [$\eta$ in Eq. (S1)] is set to 20 meV, while the electronic temperature in the Fermi-Dirac distribution functions is set to 800 K.

The adiabatic phonon frequencies and EPC matrix elements are therefore obtained by constraining the occupation functions in DFT and DFPT calculations, while the corresponding nonadiabatic results is obtained by imposing a constrain of occupations on Eq. (S1). Note that the reference phonon results for equilibrium as presented in Fig. 1(a) of the main text are adiabatic harmonic DFPT results calculated at electronic temperature of $T = 800$ K, without inclusion of phonon entropy and phonon-phonon corrections.

## S2 Phase space vs. effective coupling discussion

In the main text, we presented how even the large relative changes in the electron-phonon matrix elements for $\mathbf{q} = \Gamma$ cancel out and concluded that all the observed renormalizations of the phonon band structure and electron-phonon features are mostly induced by the modified electron phase space. The central proof of our argument is shown in Fig. S1 where we gradually move from a completely equilibrium calculation to the completely photo-excited calculation, in each of the panels changing either the equilibrium DFPT phonon frequency to the photo-excited one, the equilibrium electron-phonon matrix elements to photo-excited ones or the equilibrium electron-distribution to the photo-excited one. Let's focus on the first panel. For this calculation we use an equilibrium Fermi-Dirac distribution schematically shown in the inset. We do a DFPT calculation and obtain equilibrium phonon frequencies $\omega_\nu^{eq}(\mathbf{q})$, coupled to electrons in equilibrium via $|g_\nu^{nm}(\mathbf{k},\mathbf{q})|^2$. Then we proceed with an electron-phonon calculation and obtain a shown phonon spectral function. Let's now focus on the last panel. There we use a photo-excited distribution schematically shown in

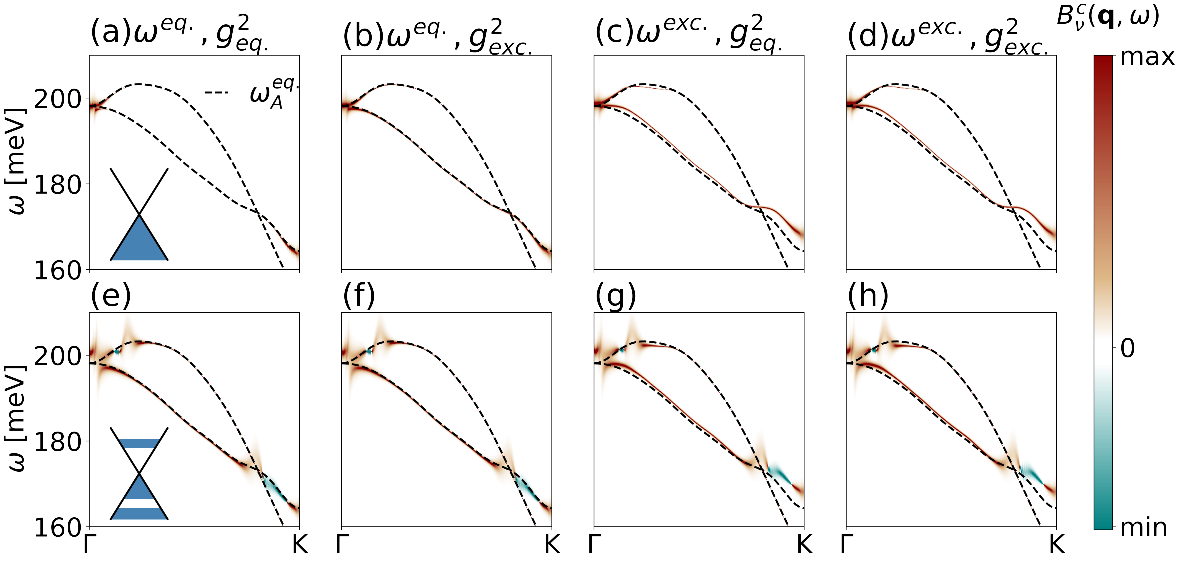


Figure S1: Spectral functions obtained by combining all possible combinations of the equilibrium and photo-excited values for the electron distribution, adiabatic DFPT frequencies and electron-phonon matrix elements. The inset in the first panel means that the whole first row is obtained with the equilibrium electron distribution, and the second row with the photo-excited one. The chosen values of the adiabatic phonon frequencies and electron-phonon matrix elements are written above each column.

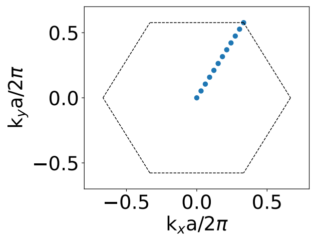


Figure S2: Chosen **q** points along the Γ-K path for which we perform the k-resolved analysis of the phonon self-energy, matrix elements and susceptibility.

the inset. We do a cDFPT calculation and obtain nonequilibrium phonon frequencies $\omega_\nu^{exc}(\mathbf{q})$, coupled to photo-excited electrons via $|g_\nu^{nm,c}(\mathbf{k},\mathbf{q})|^2$. In all the panels in between, we take all the possible combinations of equilibrium and photo-excited distributions, DFPT phonon frequencies and electron-phonon matrix elements. In the whole first row, the electron distribution is fixed to the equilibrium one (Fermi-Dirac), while in the second, it is fixed to the photo-excited distribution (see Eq. S2). Moving from panel (a) to (b) [or from (e) to (f)], the electron-phonon matrix elements are

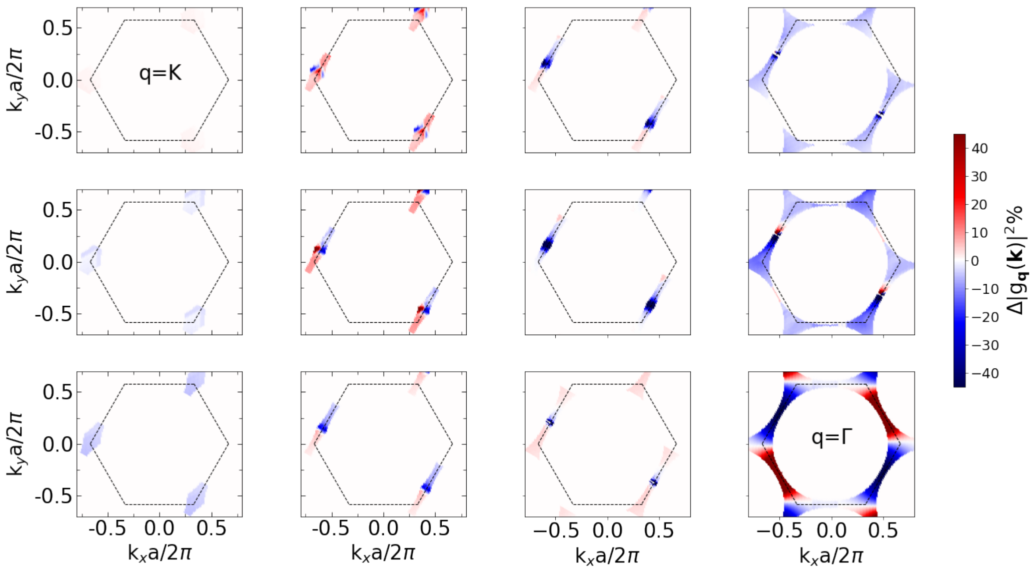


Figure S3: Relative change of the electron-phonon matrix elements $\Delta^{rel}|g_{\nu=6}(\mathbf{k})|^2$ between the photo-excited and equilibrium case.

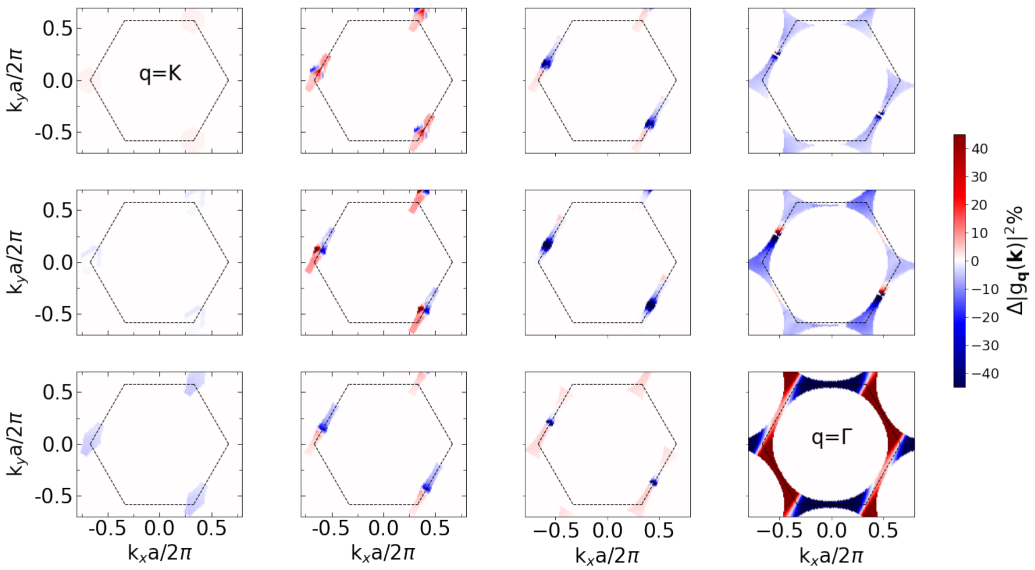


Figure S4: Relative change of the electron-phonon matrix elements $\Delta^{rel}|g_{\nu=6}(\mathbf{k})|^2$ between the photo-inverted and equilibrium case.

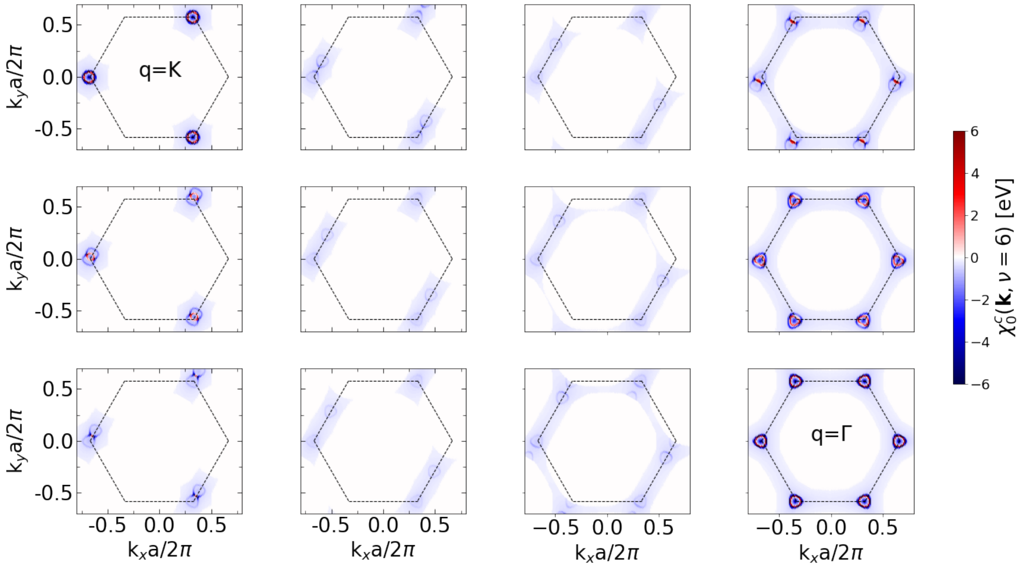


Figure S5: Bare susceptibility for the case of the photo-excited electron distribution for various q points along the Γ-K path.

changed from their equilibrium values to their photo-excited values, while the phonon frequencies are the ones obtained from an equilibrium DFPT calculation. We don't observe any significant difference between these two panels, when $|g_{\nu}^{nm}(\mathbf{k},\mathbf{q})|^2$ are exchanged by $|g_{\nu}^{nm,c}(\mathbf{k},\mathbf{q})|^2$. The same applies to the two other pairs of panels [i.e., (c-d) and (g-h)], calculated with a photo-excited phonon frequency. We observe phonon hardening around the K point which clearly derives from the adiabatic cDFPT photo-excited frequencies and again, we don't observe any additional changes deriving from the photo-induced electron-phonon matrix elements.

Additionally, we show the **k**-resolved results of the relative changes of electron-phonon matrix elements $\Delta^{rel}|g_{\nu=6}(\mathbf{k})|^2$, susceptibility $\chi_0^c(\mathbf{k})$ and phonon self-energy $\pi^c(\mathbf{k})$ for the highest optical branch ($\nu$=6) for 12 points along the Γ-K path shown in Fig. S2. The largest relative changes for both, the photo-excited (Fig. S3) and photo-inverted (Fig. S4) distribution of electrons, occur for $\mathbf{q} = \Gamma$. When calculating the relative changes of the electron-phonon matrix elements, we take into account couplings of the electronic states to the optical phonon, which can be quite far away from the Fermi

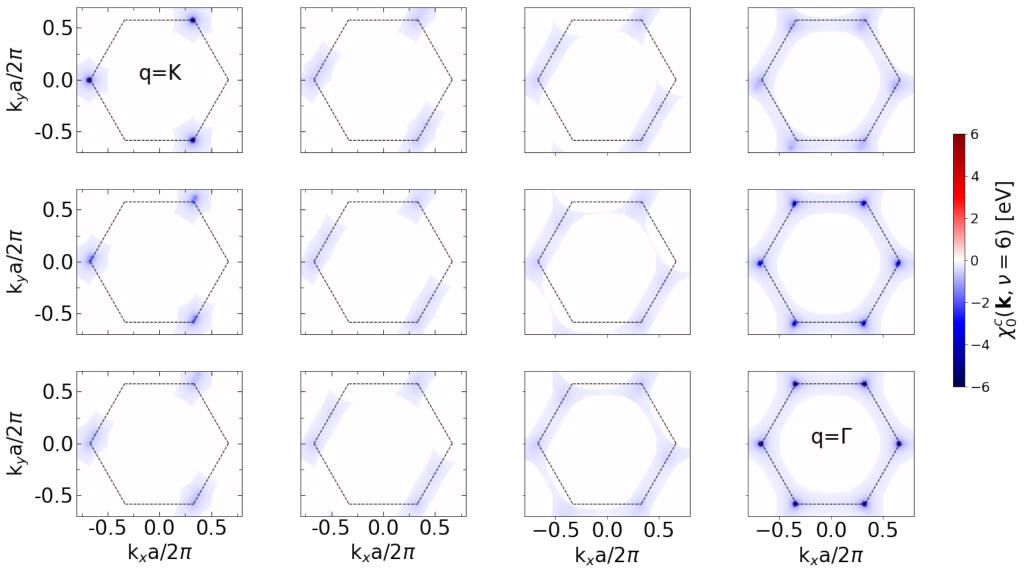


Figure S6: Bare susceptibility for the case of the photo-inverted electron distribution for various q points along the Γ-K path.

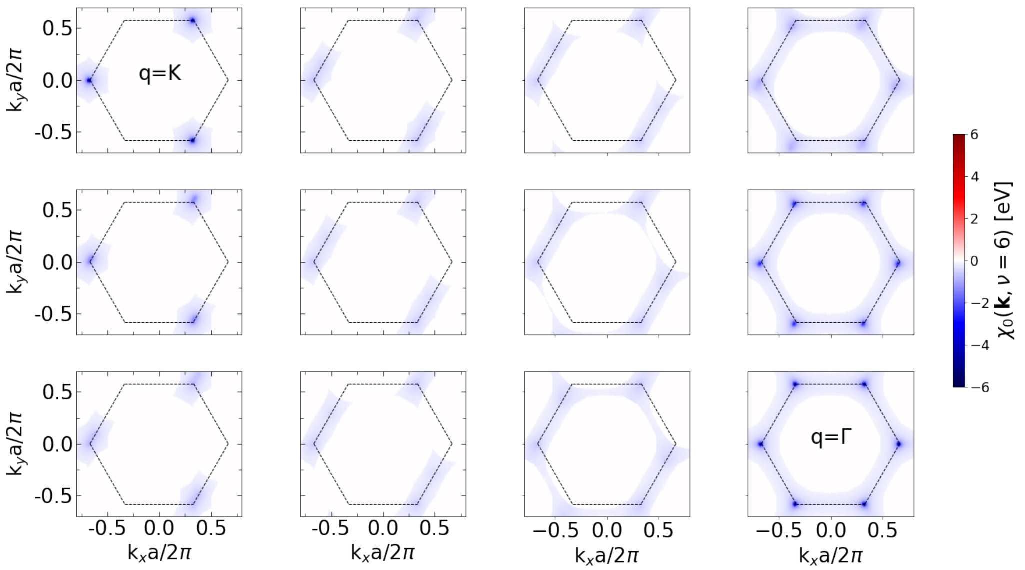


Figure S7: Bare susceptibility for the equilibrium electron distribution for various q points along the Γ-K path.

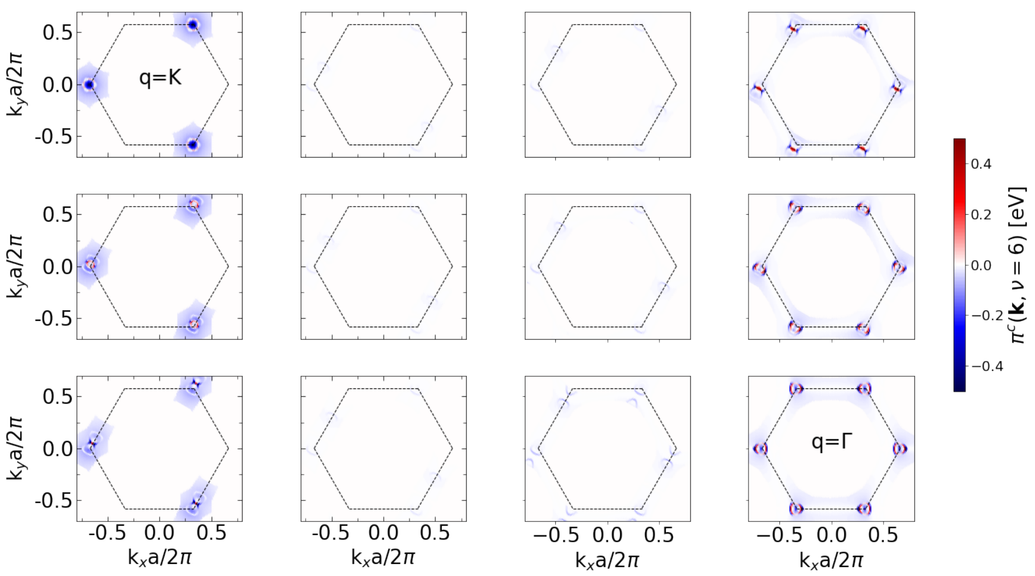


Figure S8: Phonon self-energy for the case of the photo-excited electron distribution for various q points along the Γ-K path.

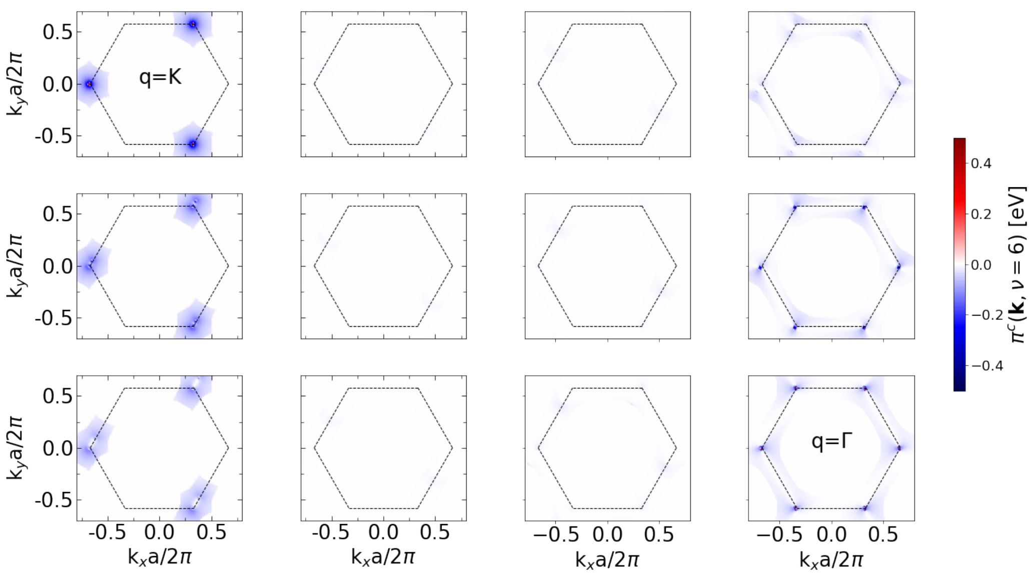


Figure S9: Phonon self-energy for the case of the photo-inverted electron distribution for various q points along the Γ-K path.

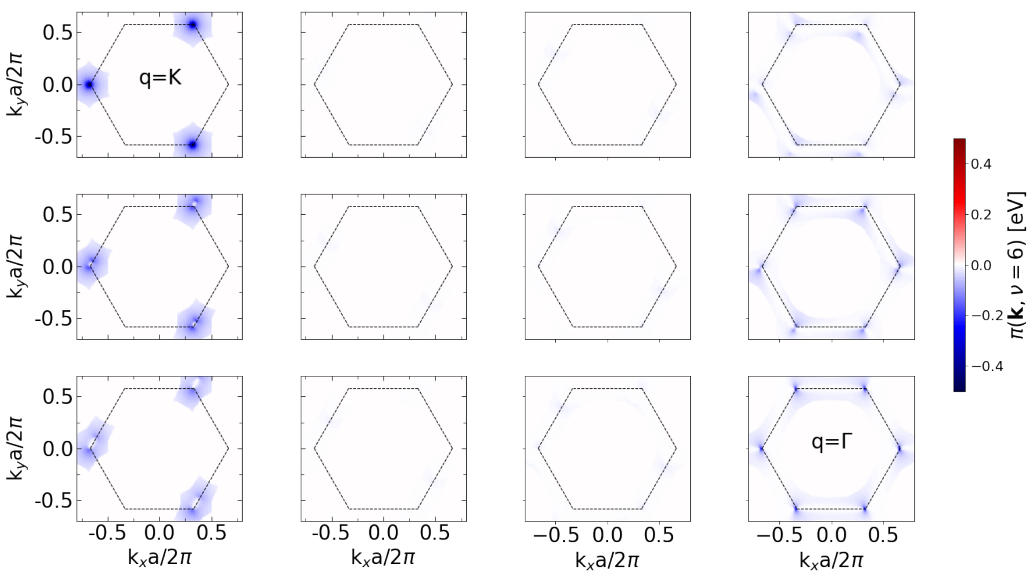


Figure S10: Phonon self-energy for the equilibrium electron distribution for various q points along the Γ-K path.

level. It can even correspond to the coupling between two full or two empty electronic states. The larger values of the relative changes of the electron-phonon matrix elements therefore also derive from the electron transitions, which have no impact on phonon spectral features. Electron-phonon matrix elements are the largest in the vicinity of $\mathbf{q} = \Gamma$ and $\mathbf{q} = \mathrm{K}$. In between, they shrink by an order of magnitude, which is why the observed relative changes in between these two end-points have no visible impact in the phonon dispersion and spectral features. On top of that, the small size of the available phase space [see $\chi_0^c(\mathbf{k})$ for the photo-excited distribution in Fig S5 and photo-inverted distribution in Fig S6] for those q-points eventually renders their $\Delta^{rel}|g_{\nu=6}(\mathbf{k})|^2$ effect negligible. We observe positive and negative $\Delta^{rel}|g_{\nu=6}(\mathbf{k})|^2$, in various parts of the BZ. When multiplied with the susceptibility factor $\chi_0^c(\mathbf{k})$ (see Figs. S5 and S6), positive and negative contributions are symmetrically picked out. They then cancel each other out, making the net effects of $\Delta^{rel}|g_{\nu=6}(\mathbf{k})|^2$ insignificant, eventually leading to results such as in Fig. S1. In Fig S7 we show the equilibrium susceptibility $\chi_0(\mathbf{k})$ for comparison. The last three pictures are $\mathbf{k}$-resolved phonon self-energies for the photo-excited (Fig. S8), photo-inverted (Fig. S9) and equilibrium (Fig. S10) electron distribution.

Even though we observe significant relative changes in the matrix elements all along the Γ - K path, when electron-phonon matrix elements are multiplied by the $\chi_0^c(\mathbf{k})$ factor, we obtain very small phonon self-energy. The more significant values of the phonon self-energy correspond to the regions in close proximity to the $\mathbf{q} = \Gamma$ and $\mathbf{q} = K$ points due to finite coupling elements and available phase space. The net effect of the dynamic self-energy renormalizations is therefore visible only around $\mathbf{q} = \Gamma$ and $\mathbf{q} = K$. From this discussion, it is important to distinguish three reasons which eventually make phase space the leading mechanism for the observed phonon spectral features: (i) A symmetric nature of the susceptibility factor $\chi_0^c(\mathbf{k})$ together with the fact that for some k points, our calculations show a photo-induced reduction or enhancement of electron-phonon matrix elements, means that these photo-induced changes in the $|g_{\nu=6}(\mathbf{k})|^2$ cancel out. This argument is important for $\mathbf{q} = \Gamma$. (ii) Due to a very small phase space for electron transitions for q points in between Γ and K as well as weak coupling to electrons, the phonon self-energy practically vanishes. Even though we do observe significant $\Delta^{rel}|g_{\nu=6}(\mathbf{k})|^2$ there, they are meaningless in our calculations. (iii) The large $\Delta^{rel}|g_{\nu=6}(\mathbf{k})|^2$ contain combinations of band indices and $\mathbf{k}$ and $\mathbf{q}$ vectors which can correspond to unphysical electron transitions (both states full/empty) or transitions with very large energy. These contributions are cut out when one takes a product with the electron susceptibility, which contains information about the available phase space.

## Supporting References


(S1) Giustino, F. Electron-phonon interactions from first principles. *Rev. Mod. Phys.* **2017**, *89*, 015003.

(S2) Page, A. F.; Ballout, F.; Hess, O.; Hamm, J. M. Nonequilibrium plasmons with gain in graphene. *Phys. Rev. B* **2015**, *91*, 075404.

(S3) Park, S.; Sammon, M.; Mele, E.; Low, T. Plasmonic gain in current biased tilted Dirac nodes. *Nat. Commun.* **2022**, *13*, 7667.

(S4) Baroni, S.; de Gironcoli, S.; Dal Corso, A.; Giannozzi, P. Phonons and related crystal properties from density-functional perturbation theory. *Rev. Mod. Phys.* **2001**, *73*, 515.

(S5) Giannozzi, P. et al. Advanced capabilities for materials modelling with QUANTUM ESPRESSO. *J. Phys. Condens. Matter* **2017**, *29*, 465901.

(S6) Berges, J.; van Loon, E. G. C. P.; Schobert, A.; Rösner, M.; Wehling, T. O. Ab initio phonon self-energies and fluctuation diagnostics of phonon anomalies: Lattice instabilities from Dirac pseudospin physics in transition metal dichalcogenides. *Phys. Rev. B* **2020**, *101*, 155107.

(S7) Novko, D. Broken adiabaticity induced by Lifshitz transition in $MoS_2$ and $WS_2$ single layers. *Commun. Phys.* **2020**, *3*, 1.

(S8) Poncé, S.; Margine, E.; Verdi, C.; Giustino, F. EPW: Electron–phonon coupling, transport and superconducting properties using maximally localized Wannier functions. *Comput. Phys. Commun.* **2016**, *209*, 116.

(S9) van Setten, M. J.; Giantomassi, M.; Bousquet, E.; Verstraete, M. J.; Hamann, D. R.; Gonze, X.; Rignanese, G. M. The PseudoDojo: Training and grading a 85 element optimized norm-conserving pseudopotential table. *Comput. Phys. Commun.* **2018**, *226*, 39.

(S10) Marzari, N.; Mostofi, A. A.; Yates, J. R.; Souza, I.; Vanderbilt, D. Maximally localized Wannier functions: Theory and applications. *Rev. Mod. Phys.* **2012**, *84*, 1419.
